# Supplementary material for: Computing Optimal Coarse Correlated Equilibria in Sequential Games
Source: arXiv:1901.06221 source file (2019-01-18)
Supplement: Supplementary file 1 [file appendix.tex]

\appendix

\section{CE and CCE: an Example}

A coarse correlated equilibrium my not be a correlated equilibrium. Moreover, an optimal CCE may lead to a social welfare arbitrarily larger than the social welfare provided by the optimal CE on the same game. Figure~\ref{fig:example} reports a normal-form game where this happens ($k > 1$).

\begin{figure}[h!]
			\centering
			\begin{tabular}{r|c|c|c|}
				\multicolumn{1}{r}{}
				&  \multicolumn{1}{c}{$a_2^1$}
				& \multicolumn{1}{c}{$a_2^2$}
				& \multicolumn{1}{c}{$a_2^3$}\\
				\cline{2-4}
				$a_1^1$ & $k,0$ & $-k^2,0$ & $-k^2,1$ \\
				\cline{2-4}
				$a_1^2$ & $-k^2,0$ & $1,0$ & $-k^2,-1$\\
				\cline{2-4}
			\end{tabular}
			\caption{Example on the difference between CE and CCE.}
			\label{fig:example}
\end{figure}

The joint strategy profile assigning probability $1/2$ to $(a_1^1,a_2^1)$ and $(a_1^2,a_2^2)$ is the CCE maximizing the social welfare of the players, which is $(k+1)/2$. The unique optimal CE is the probability distribution assigning probability 1 to $(a_1^2,a_2^2)$, providing a social welfare of 1 independently of $k$. Therefore, for increasing values of $k$, an optimal CCE allows the players to reach a social welfare which is arbitrarily larger than the social welfare reached through the optimal CE.

\section{Omitted Proofs}\label{sec:omitted}

\backward*

\noindent\textbf{Proof}.
Let us focus on the case in which we look for $p_2\in P_2$. First, define $\bar{U}_1$ s.t. $\bar{U}_1(q_1,q_2):=\zeta(q_1)U_1(q_1,q_2)$ for each $(q_1,q_2)\in Q_1\times Q_2$. Then, let $\bar{\Gamma}$ be the extensive-form game obtained from $\Gamma$ by substituting player 1's utility function with $\bar{U}_1$. Given $\bar{\Gamma}$, denote by $(q_1^\ell,q_2^\ell)$ the pair of sequences identifying $\ell$, and by $H_i^\ell$ the set of information sets of player $i$ encountered in sequence $q_i^\ell$. Algorithm~\ref{alg:backward} returns the set of actions ($A'_i$) forming a plan of the normal-form game (not reduced) equivalent to $\bar{\Gamma}$. 

\begin{algorithm}
	\caption{\texttt{Constrained-plan-search}}
	\begin{scriptsize}
		\begin{algorithmic}[1]
			\Function{C-PLAN-SEARCH}{$x$, $\bar{\Gamma}$, $i$, $q_i^\ell$, $H_i^\ell$, $A'_i$}\Comment{$i$ is the player for which we want to find a plan, $A'_i$ is the temporary set (initially empty) of actions of $i$ selected}
			\State $\nu \leftarrow K$\Comment{$K$ is a sufficiently large constant}
			\State $a'\leftarrow$null
			\If{$x$ is terminal}
			\State \textbf{return} $(\bar{U}_{-i}(x),A'_i)$
			\Else
			\If{$x\in V_{-i}$}
			\For {$y\in x.\textnormal{child}$}
			\State $\nu +=\textnormal{C-PLAN-SEARCH}(y,\bar{\Gamma},i,q_i^\ell,H_i^\ell,A'_p).\textnormal{val}$
			\EndFor
			\State \textbf{return} $(\nu,A'_i)$
			\Else 
			\If{$\exists h \in H_i^\ell: x \in h$}
			\State $a'\leftarrow$ action specified by $q_i^\ell$
			\State $y_{a'}\leftarrow$ child of $x$ reached through $a'$
			\State $\nu=\textnormal{C-PLAN-SEARCH}(y_{a'},\Gamma',i,q_i^\ell,H_i^\ell,A'_i).\textnormal{val}$
			\Else
			\For{$y\in x.\textnormal{child}$} 							\State$temp\leftarrow\textnormal{C-PLAN-SEARCH}(y,\bar{\Gamma},i,q_i^\ell,H_i^\ell,A'_i)$
			\If{$temp.\textnormal{val}<\nu$}
			\State $\nu\leftarrow temp.\textnormal{val}$
			\State $a'\leftarrow a\in\rho(x): \chi(x,a)=y$
			\EndIf
			\EndFor
			\EndIf
			\State \textbf{return}$(\nu,A'_i\cup \{a'\})$
			\EndIf
			\EndIf
			\EndFunction
		\end{algorithmic}
	\end{scriptsize}
	\label{alg:backward}
\end{algorithm}
To retrieve $A'_i$, Algorithm~\ref{alg:backward} performs a depth-first traversal of the tree while keeping track of the value to be minimized at each decision node ($\nu$) and selecting actions while moving backwards. Then, $p_2$ can be computed by traversing the tree from the root, and selecting actions according to those specified in $A'_2$.\hfill$\Box$

\sep*
\noindent\textbf{Proof}.
%\textcolor{red}{aggiungere formulazione del duale?}
Let $\alpha_i\in \mathbb{R}$, for all $i \in N$, be the dual variables of constraints~(2), $\beta_{1} \in \mathbb{R}^{|Q_1|}$ the dual variables of constraints~(3), $\beta_{2} \in \mathbb{R}^{|Q_2|}$ the dual variables of constraints~(4), and $\gamma \in \mathbb{R}$ the dual variable of constraint~(5). With $n=2$, $\mathcal{D}$ is an LP with a number of variables ($|Q_1|+|Q_2|+3$) polynomial in the size of the tree and an exponential ($|P_1\times P_2| + |H_1| + |H_2|$) number of constraints. We show that, given a vector $\bar z = (\bar \alpha_1, \bar \alpha_2,\bar \beta_1,\bar \beta_2,\bar \gamma)$, the problem of finding a hyperplane separating $\bar z$ from the set of feasible solutions to $\mathcal{D}$ or proving that no such hyperplane exists can be solved in polynomial time. Since the number of dual constraints corresponding to primal variables $v_i$ is linear, these constraints can be checked efficiently. We are left with the problem of examining the following set of constraints, defined for all $(p_1,p_2)\in P_1\times P_2$:
\begin{multline*}
r^\mathsf{T}_{p_1}\,U_1\,r_{p_2} \bar\alpha_1 + r^\mathsf{T}_{p_1}\,U_2\,r_{p_2} \bar\alpha_2 + \bar\beta_1^\mathsf{T}\, U_1\, r_{p_2} +r_{p_1}^{\mathsf{T}}\, U_2\,\bar\beta_2+ \bar\gamma \geq\\
r_{p_1}^\mathsf{T}\,(U_1+U_2)\,r_{p_2}.%, \forall (p_1,p_2)\in P_1\times P_2.
\end{multline*}
\noindent We consider the {\em separation problem} of finding an inequality of $\mathcal{D}$ which is maximally violated at $\bar z$, which reads:
\vspace{0.1cm}
\begin{multline*}
\min_{(p_1,p_2) \in P_1 \times P_2}  \Bigg\{r^\mathsf{T}_{p_1}\left((\bar \alpha_1-1) \,U_1 + (\bar \alpha_2-1) \,U_2\right) \,r_{p_2} + \\ \bar\beta_{1}^\mathsf{T}\,U_1 \,r_{p_2}  + r_{p_1}^{\mathsf{T}}\,U_2 \,\bar \beta_{2}\Bigg\}.
\end{multline*}
\noindent A pair $p_1,p_2$ yielding a violated inequality exists if and only if the optimal solution of the separation problem is $<- \bar \gamma$.

One such pair (if any) can be found in polynomial time by enumerating over the (polynomially many) possible outcomes $\ell \in L$ of the game. For each of them, we look for the pair $(p_1^\ell,p_2^\ell)$ minimizing the objective function of the separation problem, halting as soon as a pair $(p_1',p_2')$ yielding a violated constraint is found. If the procedure terminates without finding any suitable pair, we deduce that no violated inequalities exist and $\mathcal{D}$ has been solved. 
First, notice that $r^\mathsf{T}_{p_1}((\bar \alpha_1-1) U_1 + (\bar \alpha_2-1) U_2) r_{p_2}$ is constant for the family of pairs identifying $\ell\in L$. Therefore, we can consider a separate subproblem for each player (i.e., we can find $p_1^\ell$ and $p_2^\ell$ independently one from the other). Hence, for each outcome $\ell$ and for each player $i$, the corresponding $p_i^\ell$ can be found in polynomial time due to Lemma~\ref{lemma:backward}, by proceeding as described in the constructive proof of the lemma.\hfill$\Box$

\hard*
\noindent\textbf{Proof}. The construction introduced in~\cite[Theorem 1.3]{vonStengel2008} can be employed. We sketch its basic structure and apply it to the problem of solving the \textsf{NFCCE-SW} problem. The reduction is from \textsf{SAT}, whose generic instance is a Boolean formula $\phi$ in conjunctive normal form with $\eta$ clauses and $\nu$ variables. Given $\phi$, we build an auxiliary game $\Gamma_\phi$ with size proportional to that of the boolean formula. The root of $\Gamma_\phi$ is a chance node, with one action for each clause of $\phi$. Then, on the \emph{second level} of the tree, there are $\eta$ decision nodes of Player 1, each one belonging to a singleton information set and identifying a single clause of $\phi$. At each of this decision nodes, Player 1 has an action for each literal (negated or non-negated variable) appearing in the clause identified by the decision node. Player 2 plays on the \emph{third level} of the game and has a decision node for each literal appearing in $\phi$. An action of Player 1 leads to the decision node of Player 2 corresponding to the same literal. Decision nodes of Player 2 are grouped in $\nu$ information sets, one for each variable appearing in $\phi$. Each of these information sets has two available actions, corresponding to the truth assignment of the variable, and leading to a terminal node. Both players have the same payoffs, which is 0 if the literal (chosen by player 1 from the clause) is false and 1 if it is true. $\Gamma_\phi$ admits a pure strategy guaranteeing social welfare 2 if and only if $\phi$ is satisfiable. Otherwise, the maximum expected social welfare cannot be more than $2(1-1/\eta)$. Notice that a pure strategy maximizing the social welfare is also an NFCCE, since no \emph{ex-ante} deviation would result in an increase in the player's utility, being it already maximal. Then, finding a solution to \textsf{NFCCE-SW} in polynomial time would imply the existence of a polynomial time algorithm for the \textsf{SAT} problem, which leads to a contradiction unless \textsf{P}=\textsf{NP}. This concludes the proof.\hfill$\Box$

\smallskip

\noindent Notice that, when considering the separation problem of $\mathcal{D}$, working with chance is hard because the first term is no longer constant when an outcome is fixed. In the case in which $n>2$ and the game has no chance moves instead, one would have to determine the joint best-response of two player a time (for terms of the separation problem following the first one), which is \textsf{NP}-hard~\cite{vonStengel2008}.

\purificabili*

\noindent\textbf{Proof}. Realization plans $r_1^\ast$, $r_2^\ast$ already select with probability 1 sequences on the path to $\ell^\ast$ (constraint~\ref{eq:R}). In the following, we show how to find a valid $r_{p_1}^\ast$ from $r_1^\ast$, the same holds for Player 2. For each $q_1\in Q_1$, if $r_1^\ast(q_1)\in\{0,1\}$, then $r_{p_1}^\ast(q_1)=r_1^\ast(q_1)$. Now, notice that $r_1^\ast\in \textnormal{co}\left( \times_{p_1\in P_1}r_{p_1}\right)$, meaning that each realization plan can be written as $r_1=\sum_{p_1\in P_1}\delta_{p_1}r_{p_1}$, with $\delta_{p_1}\geq 0$, for each $p_1\in P_1$, and $\sum_{p_1\in P_1}\delta_{p_1}=1$. Denote by $\delta_1^\ast$ the coefficients of $r_1^\ast$. Let $r_{p_1}$ and $r_{p_1'}$ be s.t. $\delta_{p_1}^\ast,\delta_{p_1'}^\ast>0$. Optimality of $(r_1^\ast,r_2^\ast)$ implies that $r_{p_1}^\tr U_2\bar{\beta_2}<r_{p_1'}^\tr U_2\bar{\beta_2}$ is not possible. Specifically, $r_{p_1}^\tr U_2\bar{\beta_2}=r_{p_1'}^\tr U_2\bar{\beta_2}$ has to hold. Then, it is enough to set $r_{p_1}^\ast$ equal to a $r_{p_1}$ s.t. $\delta_{p_1}^\ast>0$. To find one of such plans, traverse the tree in a depth-first fashion, and select sequences, among those played with strictly positive probability in $r_1^\ast$, following the same reasoning of Algorithm~\ref{alg:backward}. Once the tree has been fully traversed, $r_{p_1}^\ast$ is built according to the selected actions. Notice that $r_{p_1}^\ast$ has to be such that $r_{p_1}^{\ast\tr} U_2\bar \beta_2=r_1^{\ast\tr} U_2\bar \beta_2$, otherwise optimality of $r_1^\ast$ given $\ell^\ast$ would be violated.
\hfill$\Box$

\section{Solving \textsf{LRC} with more than two players}

We focus on a game with $n=3$, without chance moves. The oracle can be easily adapted to the setting with $n>3$, and to include the Chance player. Denote by $U_{i,r_j}$ the utility matrix of player $i$ marginalized with respect to realization plan $r_j$ of player $j$--- notice that the $U_{i,r_j}\in \mathbb{R}^{|Q_i|\times |Q_t|}$, with $i,t\in N$, and $i,t\ne j$. The objective function that needs to be maximized is:
\begin{equation}\label{eq:3_obj}
	\begin{split}
	r_1^\mathsf{T}\left( \left( 1-\bar\alpha_1\right)U_{1,r_3}+\left( 1-\bar\alpha_2\right)U_{2,r_3}+\left( 1-\bar\alpha_3\right)U_{3,r_3}\right)r_2\\
	-\bar\beta_1^\tr U_{1,r_3}r_2 - \bar\beta_2^\tr U_{2,r_3}^\tr r_1 - \bar\beta_3^\tr U_{3,r_1}^\tr r_2
	\end{split}
\end{equation}
The first term of the objective function only depends on the choice of a single terminal node $\ell\in L$. 
The following terms can be addressed following the same reasoning we employed to adapt \textsf{MI-LRC} to the case of a two-player game with Chance.
For example, in $-\bar\beta_1^\tr U_{1,r_3}r_2$ player 2 and 3 are jointly best-responding against a fixed distribution of player 1 ($\bar\beta_1$).
%In the following, we write $U_i(\ell)$ meaning $U_i(q_1^\ell,q_2^\ell,q^\ell_3)$.  
Then, \textsf{MI-LRC} can be substituted with the following oracle:
\begin{align}
\begin{split}
	\max \bigg(r_1^\tr\big( \left( 1-\bar\alpha_1\right)U_{1,r_3}+\left( 1-\bar\alpha_2\right)U_{2,r_3}\\+\left( 1-\bar\alpha_3\right)U_{3,r_3}\big)r_2\\
	-\bar\beta_1^\tr U_{1,r_3}r_2 - \bar\beta_2^\tr U_{2,r_3}^\tr r_1 - \bar\beta_3^\tr U_{3,r_1}^\tr r_2\bigg)
	\end{split}\label{eq:3_obj}\\
&F_i r_i=f_i\qquad \forall i\in N\\
&z\in\{0,1\}^{|L|}\\
&\sum_{\ell\in L} z(\ell)=1 \label{eq:3_sum1}\\
&z_i\in\{0,1\}^{|L|}\qquad \forall i\in N \\
& R_{i,(q_i,\cdot)}z_i=1 \qquad \forall i\in N,\forall q_i\in \bar Q_i \label{eq:3_zi_R}\\
& z_i(\ell)\geq z(\ell) \qquad \forall i\in N, \forall \ell\in L \label{eq:3_zi_z}\\
& r_j\geq R_iz_i \qquad \forall i\in N,\forall j\in N\setminus\{i\} \label{eq:3_r_zi}\\
&r_i\geq 0\qquad \forall i\in N
\end{align}

\noindent The oracle employs $n+1$ $|L|$-dimensional vectors of binary variables. Vector $z$ selects a single terminal node (constraint~\ref{eq:3_sum1}), determining the value of the first term of the objective function. Each $z_i$, instead, selects the terminal nodes reachable through a certain choice of plans of the players that are best-responding against $i$ (constraint~\ref{eq:3_zi_R}). As an example, $z_1(\ell)=1$ iff $\ell$ is reachable through the chosen $(r_2,r_3)$. Realization plans are constrained to be consistent with the selected outcomes (constraint~\ref{eq:3_r_zi}). Finally, the choices in $z$ and in each $z_i$ have to be mutually consistent (constraint~\ref{eq:3_zi_z}).

\section{Goofspiel: Rules of the Game}

Two-player Goofspiel is played using three suits of a standard 52-card deck. Cards rank Ace (low), 2, $\ldots$, 10, J, Q, K (high). When scoring points, the Ace is worth 1 point, cards 2-10 their face value, Jack 11, Queen 12, and King 13.

One suit is singled out as the \emph{prizes}. The prizes are shuffled and placed between the players, with the top card turned face up. Each of the remaining suits becomes the hand of one of the players.
 
The game proceeds in a series of rounds. Each player selects a card from her hand and places it face down, keeping her choice secret from the opponent. Once both players have selected a card, they are simultaneously revealed, and the player with the highest bid wins the prize card. 
There are various tie-breaking rules. The most popular ones are discarding the prize card or splitting its value between the two players.
At this point, the cards used for bidding are discarded, and the game continues with a new prize card turned face up.

The game ends when the players terminate the cards in their hands (after 13 rounds). Players calculate their final score by summing up the value of the prize cards they won. The player with the highest final score wins.
